# Supplementary material for: FWD: Real-time Novel View Synthesis with Forward Warping and Depth
Source: arXiv:2206.08355 source file (2022-08-05)
Supplement: Supplementary file 1 [file DTU_view_dependence.tex]

\begin{figure*}
    \centering
    \begin{tabular}{c@{}c@{\hspace{0.5mm}}c@{\hspace{0.5mm}}c@{}}
    % Input views1 &Input views2 &Input views3 & Novel views 1 &Novel views 2 &Novel views 3\\
    % \text{Input View1} &
    % \text
    \includegraphics[width=0.24\textwidth]{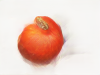}&
    \includegraphics[width=0.24\textwidth]{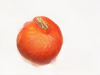}&
    \includegraphics[width=0.24\textwidth]{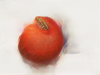}&
    \includegraphics[width=0.24\textwidth]{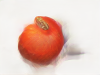}\\
    \includegraphics[width=0.24\textwidth]{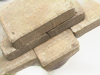}&
    \includegraphics[width=0.24\textwidth]{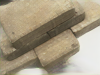}&
    \includegraphics[width=0.24\textwidth]{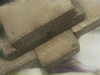}&
    \includegraphics[width=0.24\textwidth]{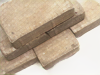}\\
    \includegraphics[width=0.24\textwidth]{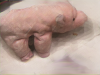}&
    \includegraphics[width=0.24\textwidth]{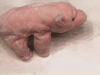}&
    \includegraphics[width=0.24\textwidth]{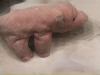}&
    \includegraphics[width=0.24\textwidth]{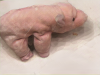}\\
    \end{tabular}
    \captionof{figure}{\textbf{The effectiveness of view-dependent feature MLP. }
    We show that for the same target views, we can get varying appearance by controlling ray difference features.
    }
    \label{fig:supp_dtu_vd}
    \end{figure*}
